# Supplementary material for: FairFace: Face Attribute Dataset for Balanced Race, Gender, and Age
Source: arXiv:1908.04913 source file (2019-08-14)
Supplement: Supplementary file 1 [file 070-SM.tex]

\begin{strip}
\centering
{
\Large
\textbf{FairFace: Face Attribute Dataset for Balanced Races} 
\\
\textbf{
Supplementary Materials}
}

\end{strip}

\\

\begin{strip}
The supplementary materials provide larger figures and tables based on the same experiments conducted in the main paper. 
\end{strip}    

%\section{Supplementary Materials} 

\begin{figure}[th!]
    \centering
      \includegraphics[width=0.9\textwidth]{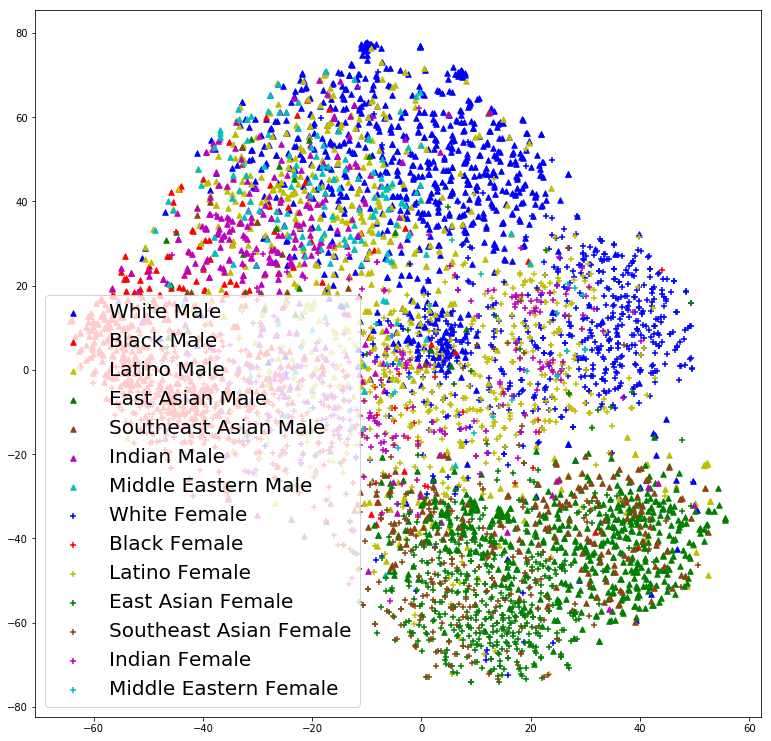}
  \caption{t-SNE visualization of sample faces in FairFace.}
\label{fig:fair-tsne}
\end{figure}

\clearpage

\begin{figure*}
\centering
      \includegraphics[width=0.9\textwidth]{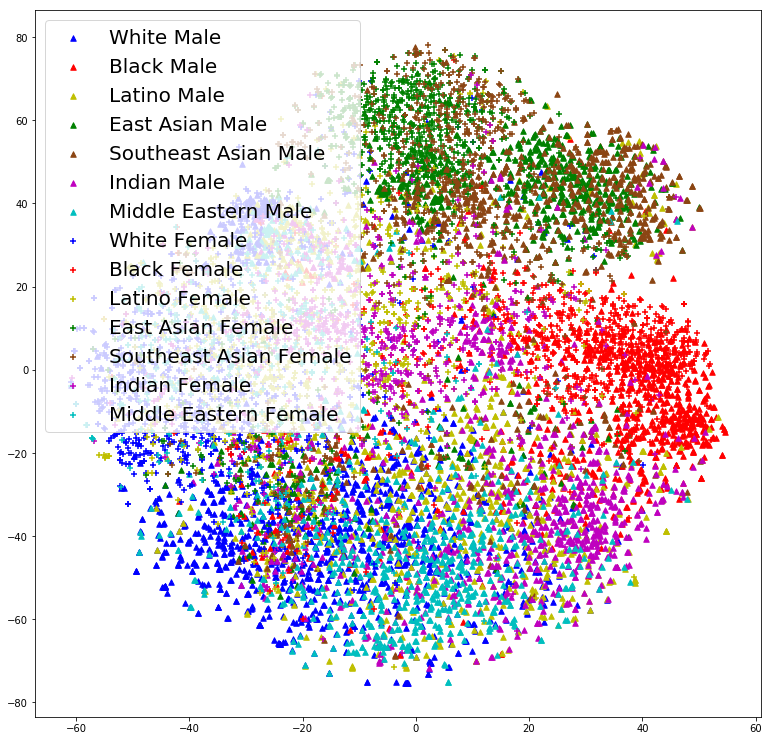}
  \caption{t-SNE visualization of sample faces in FairFace, using embeddings from the model trained on FairFace.}
\label{fig:fair-embedding-tsne}
\end{figure*}

\clearpage

\begin{figure*}
\centering
      \includegraphics[width=0.9\textwidth]{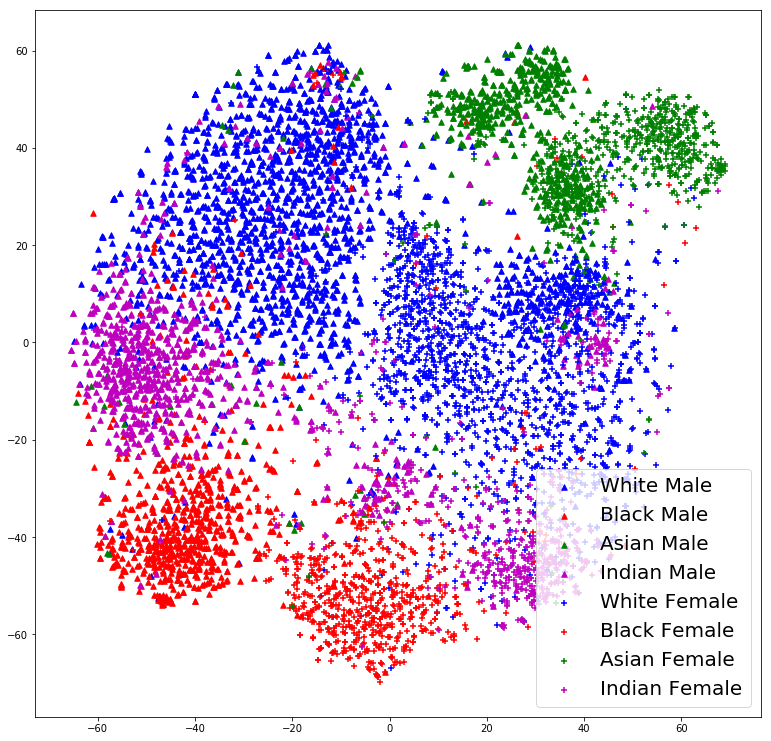}
  \caption{t-SNE visualization of sample faces in UTKFace.}
\label{fig:utk-tsne}
\end{figure*}

\clearpage

\begin{figure*}
\centering
      \includegraphics[width=0.9\textwidth]{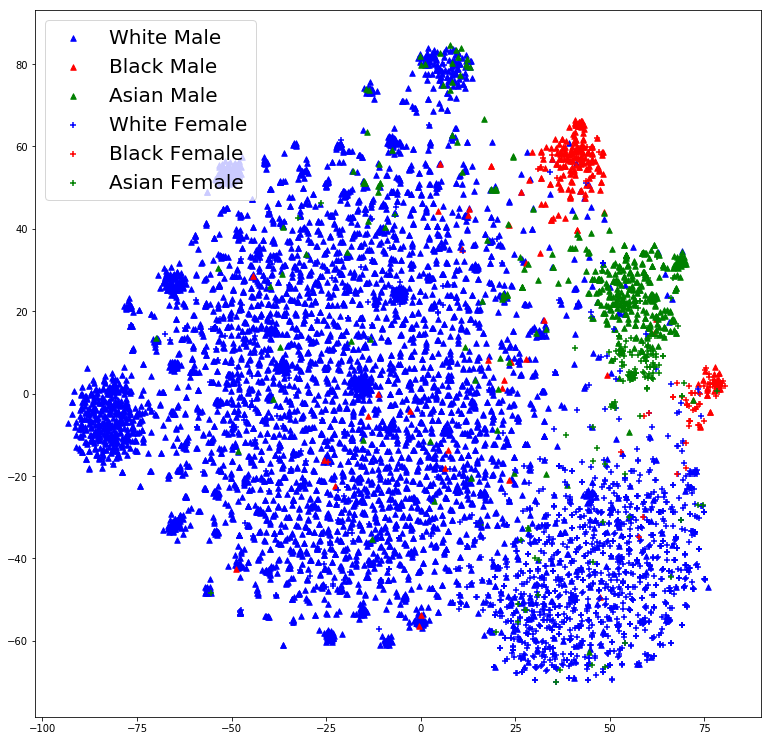}
  \caption{t-SNE visualization of sample faces in LFWA.}
\label{fig:lfwa-tsne}
\end{figure*}

\clearpage

\begin{figure*}
    \centering
    \begin{subfigure}[t]{0.33\textwidth}
    \centering
      \includegraphics[width=1\textwidth]{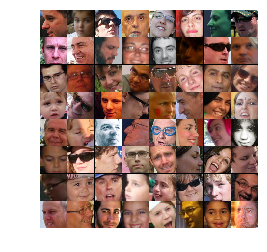}
      \caption{White}
     \end{subfigure}    ~~~
    \begin{subfigure}[t]{0.33\textwidth}
    \centering
      \includegraphics[width=1\textwidth]{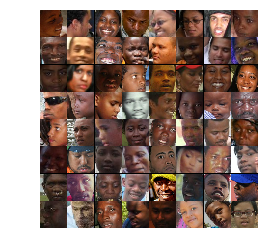}
      \caption{Black}
     \end{subfigure}    
    \begin{subfigure}[t]{0.33\textwidth}
    \centering
      \includegraphics[width=1\textwidth]{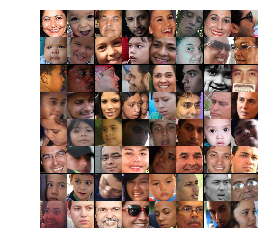}
      \caption{Latino}
     \end{subfigure}    ~~~
    \begin{subfigure}[t]{0.33\textwidth}
    \centering
      \includegraphics[width=1\textwidth]{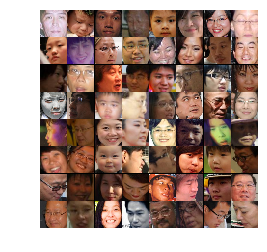}
      \caption{East Asian}
     \end{subfigure}    
    \begin{subfigure}[t]{0.33\textwidth}
    \centering
      \includegraphics[width=1\textwidth]{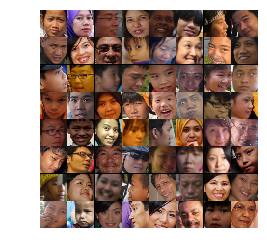}
      \caption{Southeast Asian}
     \end{subfigure}  
    \begin{subfigure}[t]{0.33\textwidth}
    \centering
      \includegraphics[width=1\textwidth]{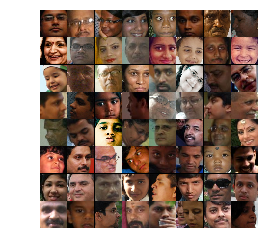}
      \caption{Indian}
     \end{subfigure}   
    \begin{subfigure}[t]{0.33\textwidth}
    \centering
      \includegraphics[width=1\textwidth]{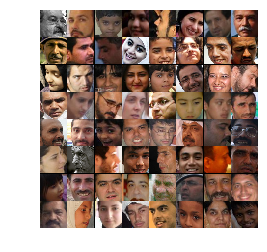}
      \caption{Middle Eastern}
     \end{subfigure}   
  \caption{Random samples from FairFace, divided by race groups.}
\label{fig:sample_fair}
\end{figure*}

\iffalse
\clearpage

\begin{figure*}
    \centering
\vspace{-10pt}
    \begin{subfigure}[t]{0.9\textwidth}
    \centering
      \includegraphics[width=1\textwidth]{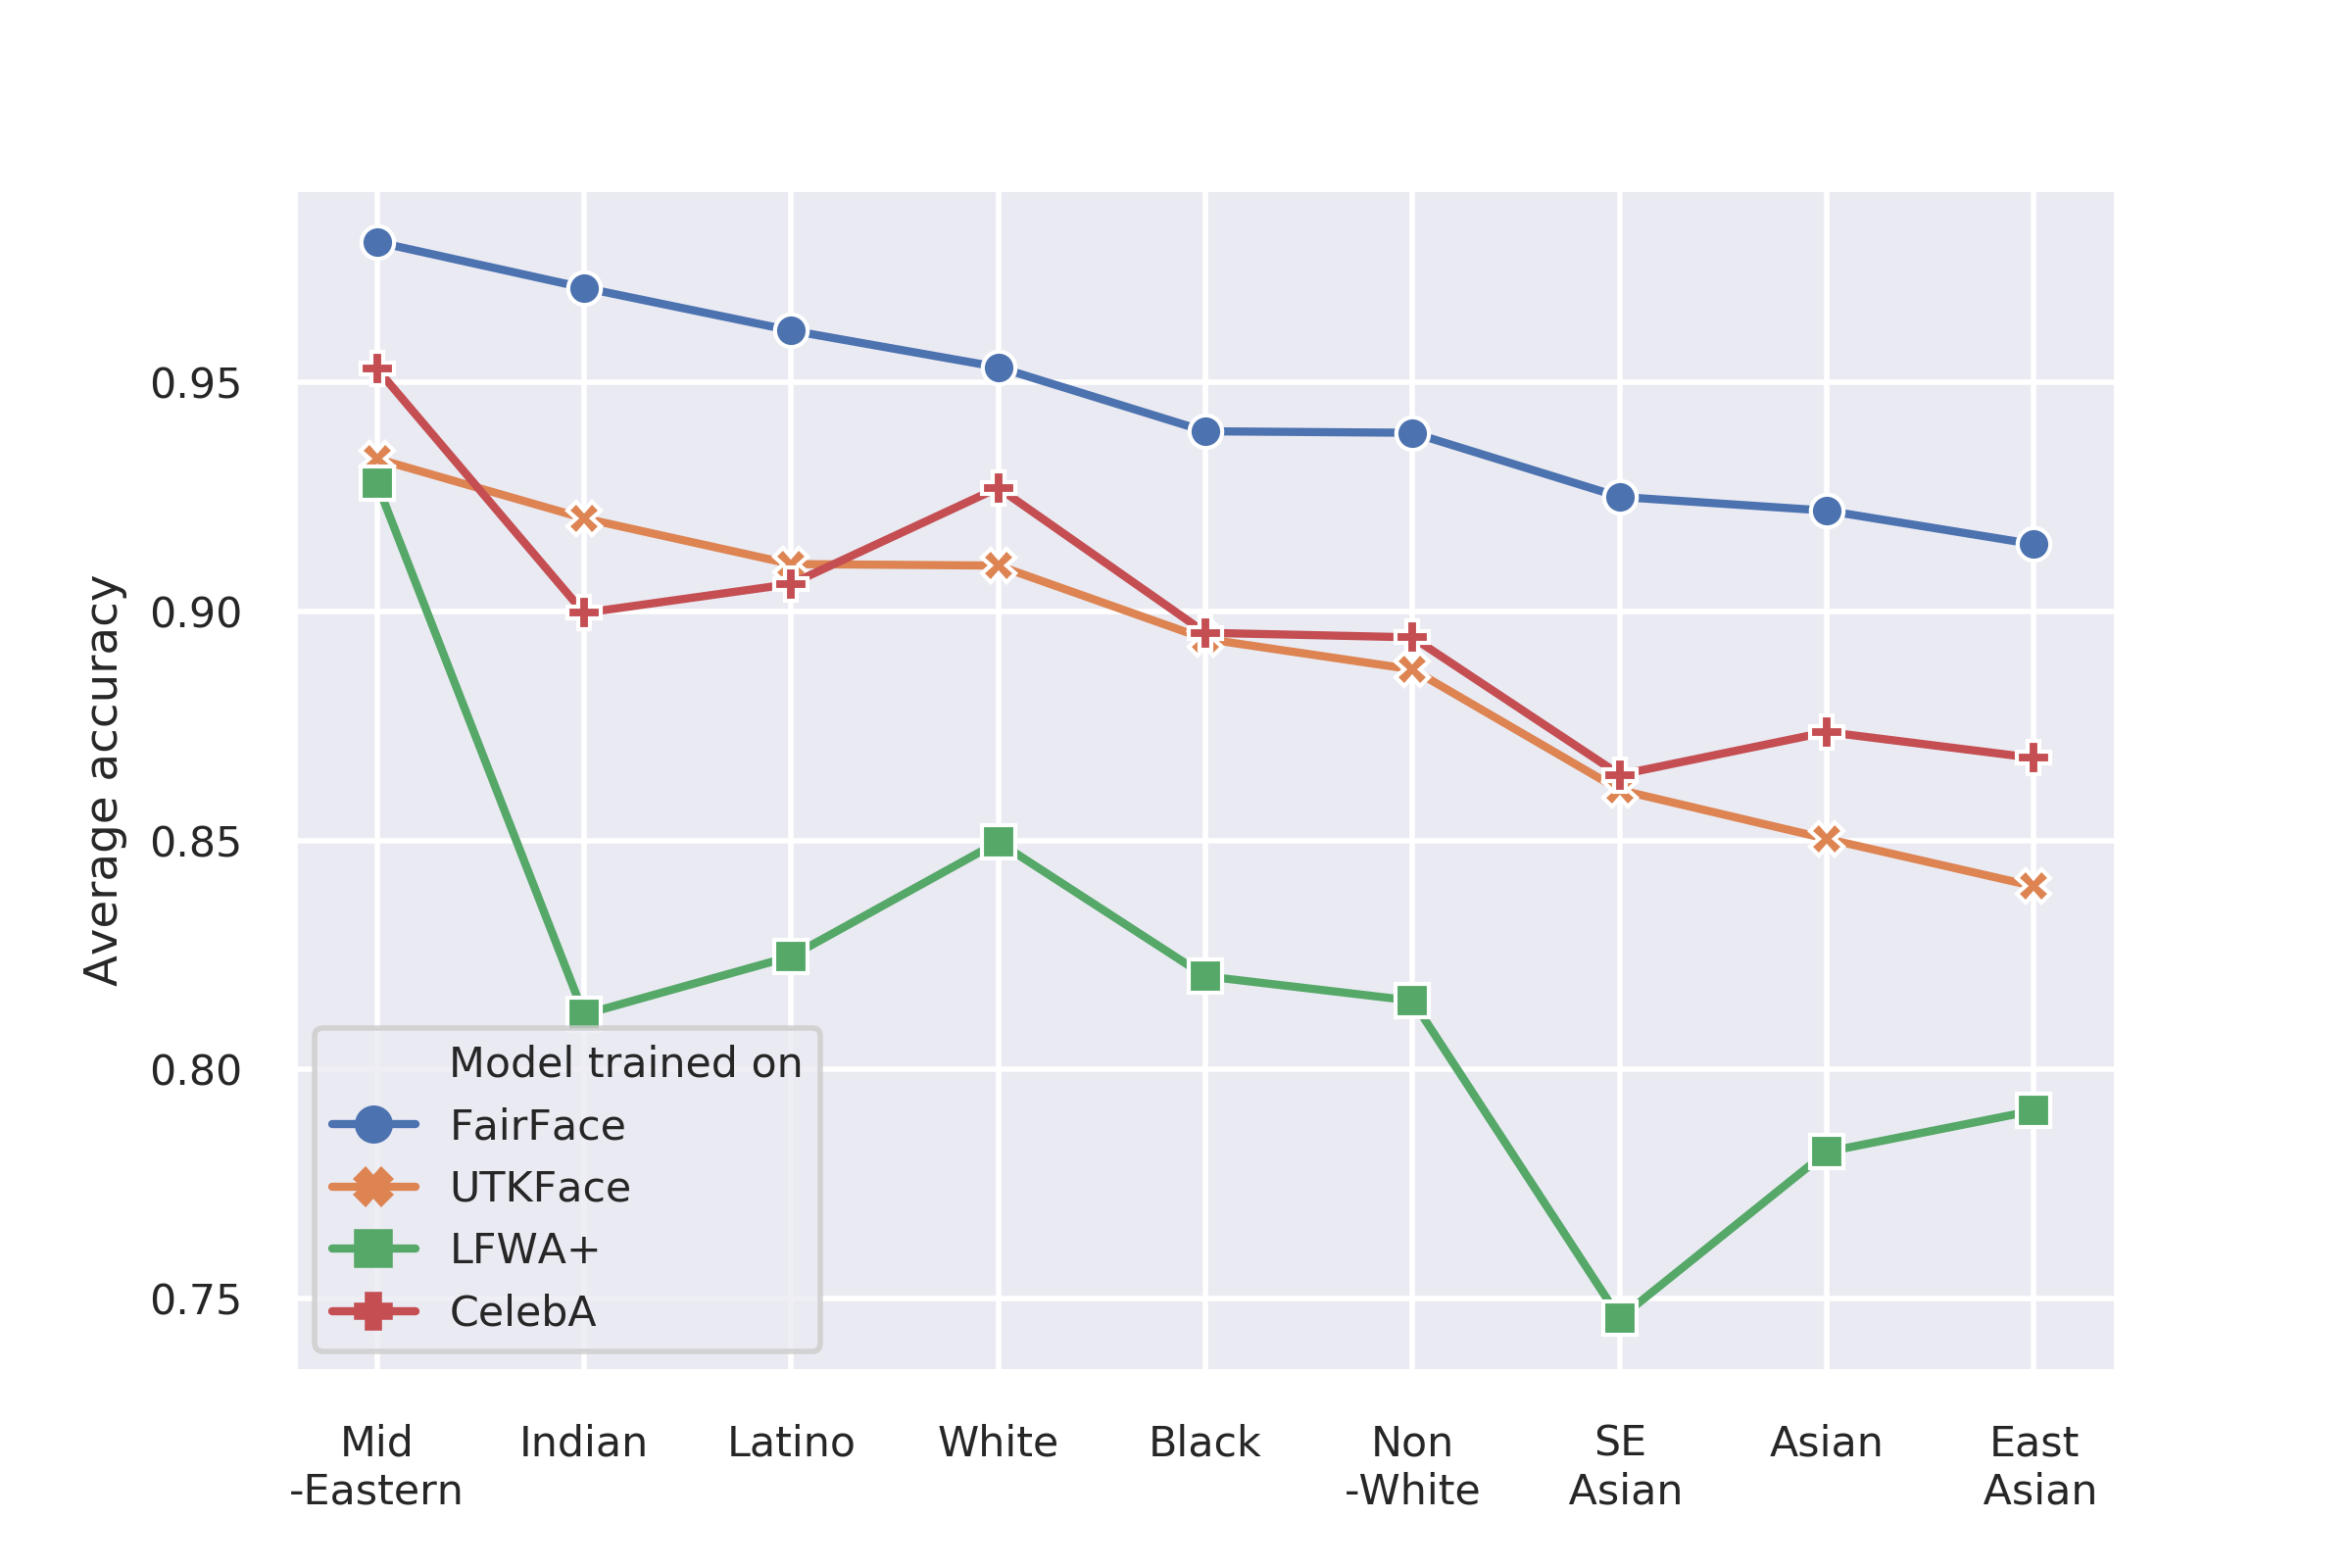}
\vspace{-20pt}
      \caption{Race groups}
     \end{subfigure}
    \begin{subfigure}[t]{0.9\textwidth}  \centering
      \includegraphics[width=1\textwidth]{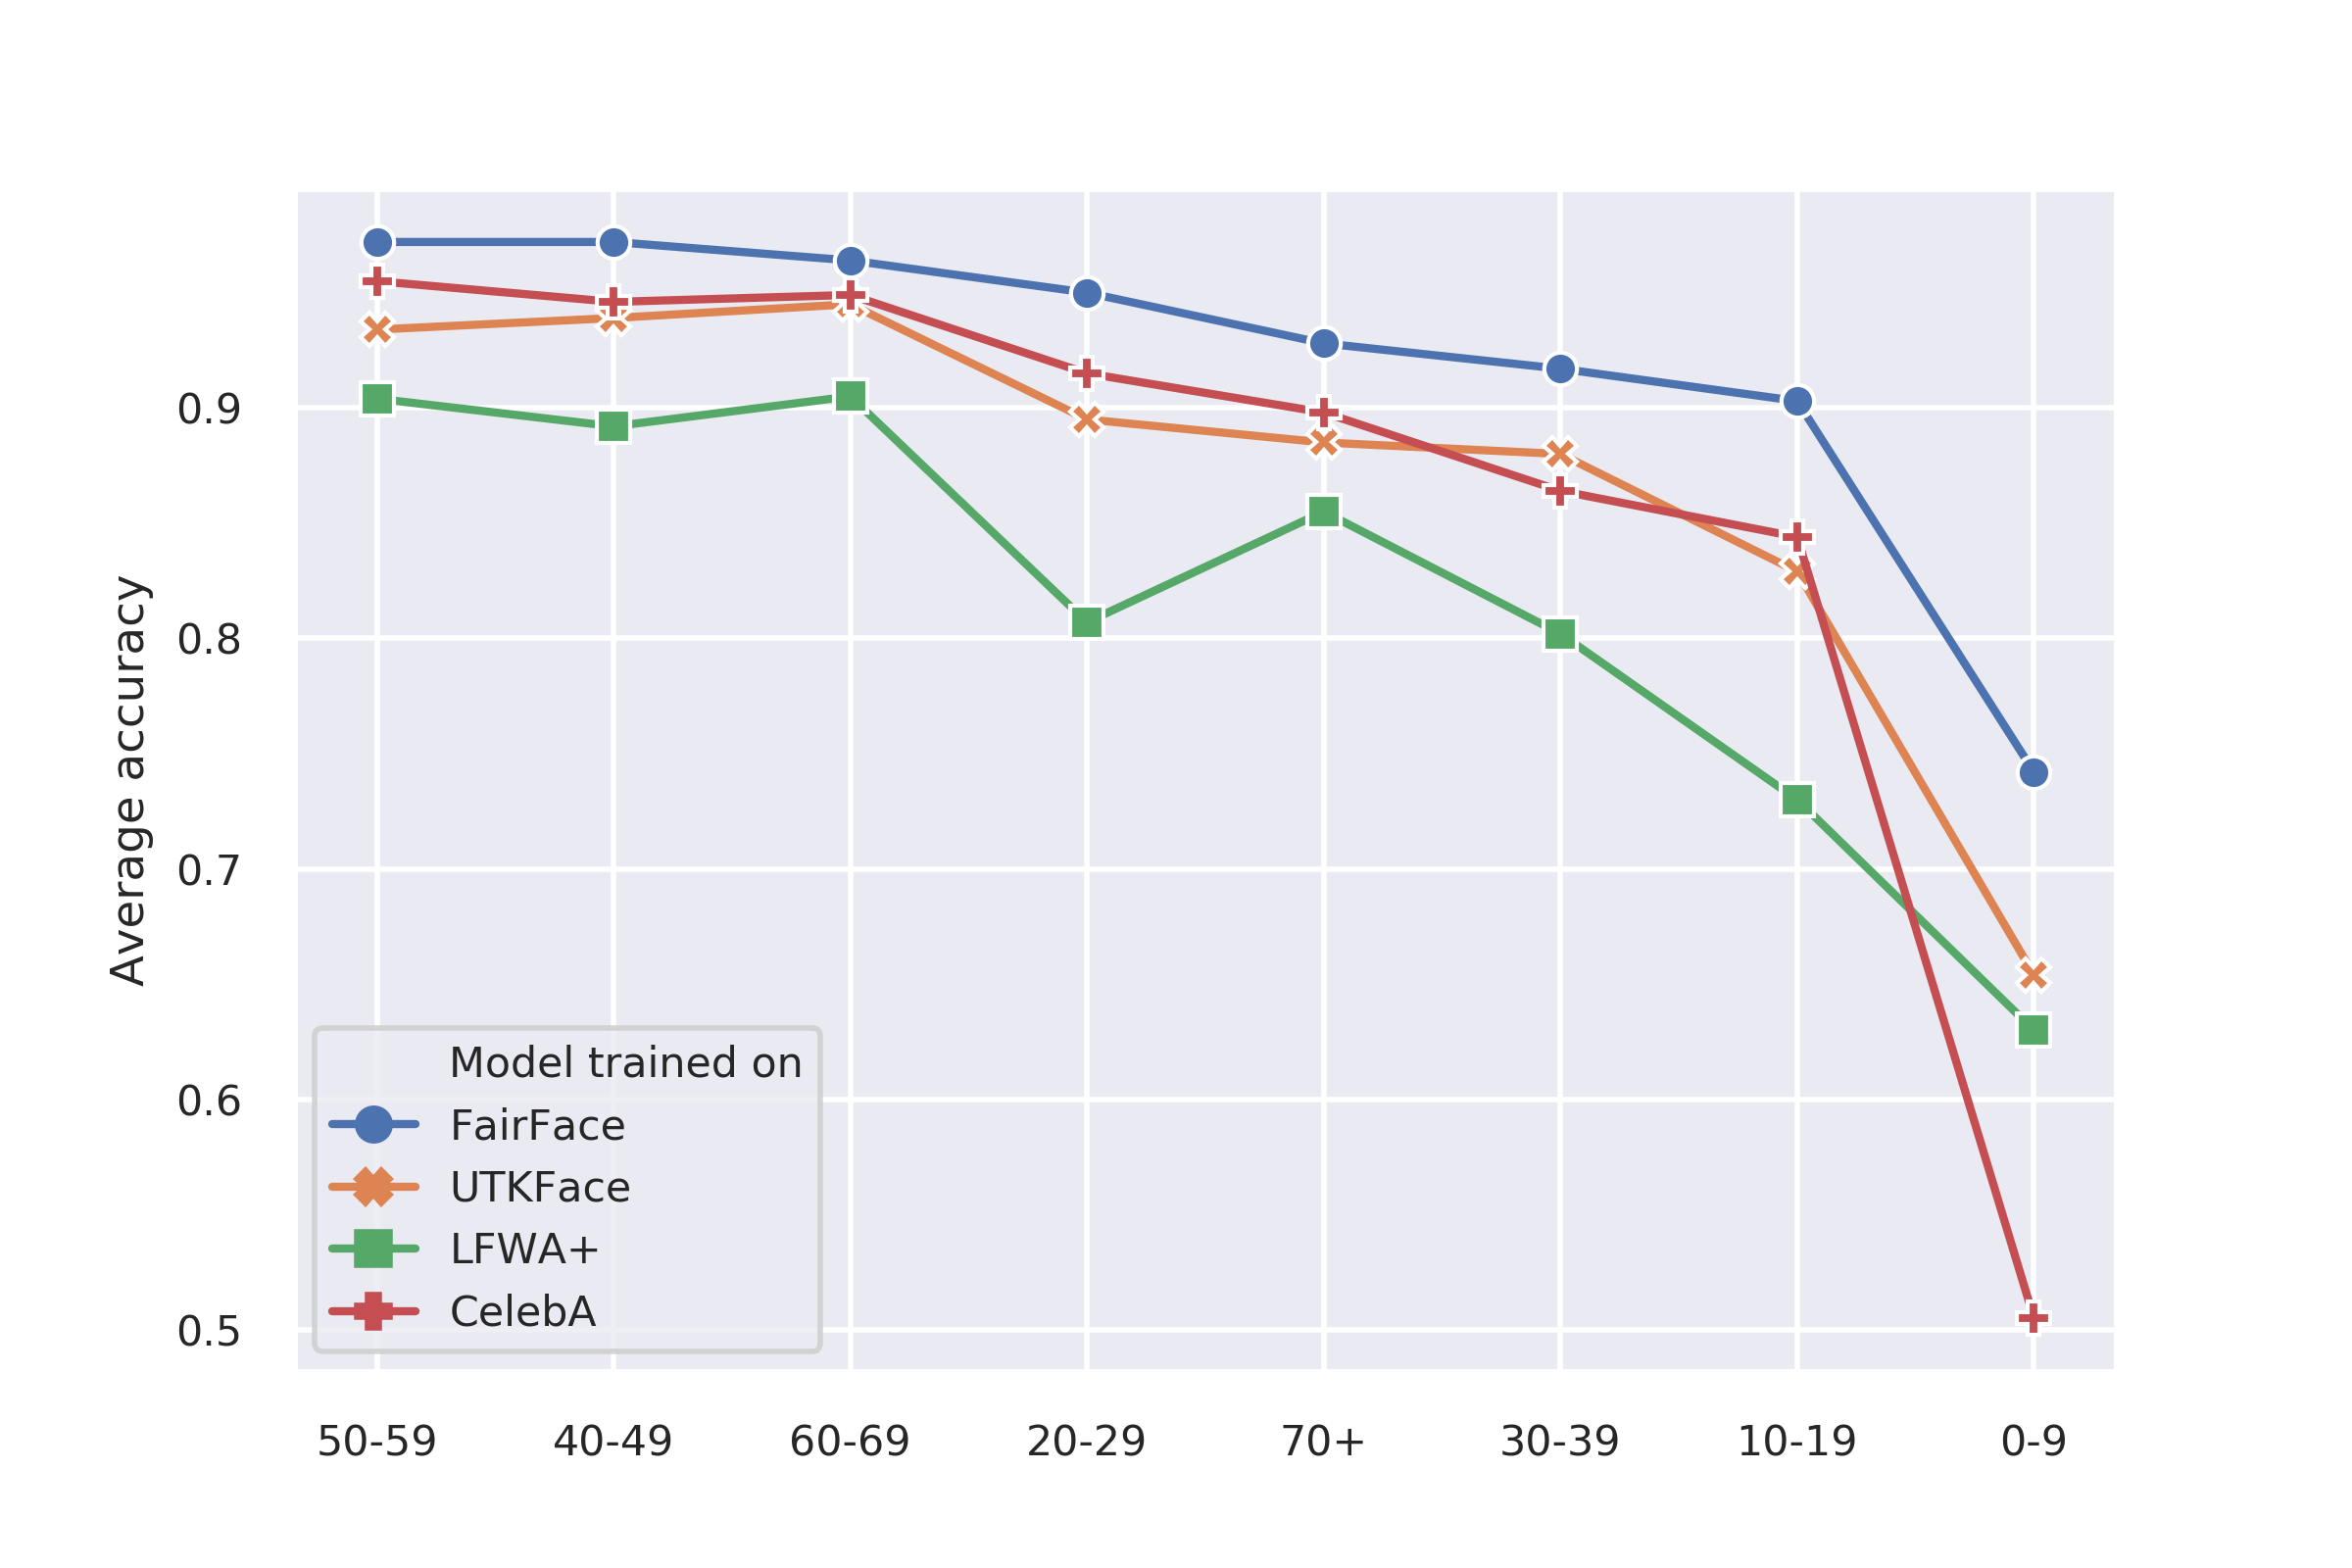}
\vspace{-20pt}
      \caption{Age groups}
     \end{subfigure}
  \caption{Average gender classification accuracy on validation datasets, divided by sub-demographics.}
\label{fig:gender_comp}
\end{figure*}
\fi

\clearpage
